# Supplementary material for: First-order Temporal Logic on Finite Traces: Semantic Properties, Decidable Fragments, and Applications
Source: arXiv:2202.00610 source file (2022-02-01)
Supplement: Supplementary file 1 [file 9-appendix.tex]

\appendix
\section{Appendix}
\label{sec:app_der}

\begin{equation}
\vdash \Next \p \rightarrow \Wnext \p
\label{eq:nexttownext}
%\tag{\ref{eq:nexttownext}}
\end{equation}
\begin{enumerate}
[label=$(\roman*)$, align=left, leftmargin=*, labelsep=*, itemindent=*]
	\item $\Box \bot \lor \Next \p \to \Wnext \p$ \hfill (\ref{eq:wnextdef}, FOL)
	\item $\Next \p \to \Wnext \p$ \hfill ($i$, FOL)
\end{enumerate}

\begin{equation*}
\vdash \Box \bot \leftrightarrow \lnot \Next \top
\tag{\ref{eq:lastequiv}}
\end{equation*}
\begin{enumerate}
[label=$(\roman*)$, align=left, leftmargin=*, labelsep=*, itemindent=*]
	\item $\Box \bot \to \Wnext \bot \land \Wnext \Box \bot$ \hfill (\ref{eq:boxdef}, FOL)
	\item $\Wnext \bot \to \lnot \Next \top$ \hfill (Def.~$\Wnext$)
	\item $\Box \bot \to \lnot \Next \top$ \hfill ($i$, $ii$, FOL)
	\item $\bot \to \Box \bot$ \hfill  (FOL)
	\item $\Box (\bot \to \Box \bot)$ \hfill ($iv$, \ref{eq:boxNec})
	\item $\Box (\bot \to \Box \bot) \to \Wnext (\bot \to \Box \bot)$ \hfill (\ref{eq:boxdef}, FOL)
	\item $\Wnext (\bot \to \Box \bot) \to (\Wnext \bot \to \Wnext \Box \bot)$ \hfill (\ref{eq:wnextK}, FOL)
	\item $\Box (\bot \to \Box \bot) \to (\Wnext \bot \to \Wnext \Box \bot)$ \hfill ($vi$, $vii$, FOL)
	\item $\Wnext \bot \to \Wnext \Box \bot$ \hfill ($v$, $viii$, FOL)
	\item $\lnot \Next \top \to \Wnext \Box \bot$ \hfill ($ix$, Def.~$\Wnext$, FOL)
	\item $\lnot \Next \top \to \Wnext \bot$ \hfill (Def.~$\Wnext$, FOL)
	\item $\lnot \Next \top \to \Wnext \bot \land \Wnext \Box \bot$ \hfill ($x$, $xi$, FOL)
	\item $\Wnext \bot \land \Wnext \Box \bot \to \Box \bot$ \hfill (\ref{eq:boxdef}, FOL)
	\item $\lnot \Next \top \to \Box \bot$ \hfill ($xii$, $xiii$, FOL)
	\item $\Box \bot \leftrightarrow \lnot \Next \top$ \hfill ($iii$, $xiv$, FOL)
\end{enumerate}

%Derivation of
%~(\ref{eq:nexttonotlast})
%$\Next \p \rightarrow \lnot \Box \bot$ \\
%
\begin{equation}
\vdash \Next \p \rightarrow \lnot \Box \bot
\label{eq:nexttoboxbot}
\end{equation}
\begin{enumerate}
[label=$(\roman*)$, align=left, leftmargin=*, labelsep=*, itemindent=*]
	\item $\Next \p \rightarrow \bot \Until \p$ \hfill (Def.~$\Next$)
	\item $\bot \Until \p \rightarrow  \Diamond \p$ \hfill $(\ref{eq:untiltodiam})$ 
	\item $\Diamond \p \rightarrow \lnot \Box \lnot \p$ \hfill (Def.~$\Box$, FOL)
	\item $\bot \to \lnot \p$ \hfill (FOL)
	\item $\Box (\bot \to \lnot \p)$ \hfill ($iv$, $\ref{eq:boxNec}$)
	\item $\Box (\bot \to \lnot \p) \to (\Box \bot \to \Box \lnot \p)$ \hfill $(\ref{eq:boxK})$
	\item $\Box \bot \to \Box \lnot \p$  \hfill ($v$, $vi$, FOL)
	\item $\lnot \Box \lnot \p \to \lnot \Box \bot$ \hfill ($vii$, FOL)
	\item $\Next \p \to \lnot \Box \bot$ \hfill ($i$-$iii$, $viii$, FOL)
\end{enumerate}

\begin{equation}
\vdash \Wnext (\p \land \psi) \rightarrow \Wnext \p \land \Wnext \psi
\label{eq:wnextandleft}
\end{equation}
\begin{enumerate}
[label=$(\roman*)$, align=left, leftmargin=*, labelsep=*, itemindent=*]
	\item $(\p \land \psi) \rightarrow  \p$ \hfill (FOL)
	\item $\Wnext ( (\p \land \psi) \rightarrow  \p)$ \hfill ($i$, $\ref{eq:wnextNec}$)
	\item $\Wnext(\p \land \psi) \rightarrow \Wnext \p$ \hfill ($ii$, $\ref{eq:wnextK}$)
	\item $(\p \land \psi) \rightarrow  \psi$ \hfill (FOL)
	\item $\Wnext ( (\p \land \psi) \rightarrow  \psi)$ \hfill ($iv$, $\ref{eq:wnextNec}$) 
	\item $\Wnext(\p \land \psi) \rightarrow \Wnext \psi$ \hfill ($v$, $\ref{eq:wnextK}$)
	\item $\Wnext(\p \land \psi) \rightarrow \Wnext \p \land \Wnext \psi$ \hfill ($iii$, $vi$, FOL)
\end{enumerate}

\begin{equation}
\vdash \Wnext \p \land \Wnext \psi \rightarrow \Wnext (\p \land \psi)
\label{eq:wnextandright}
\end{equation}
\begin{enumerate}
[label=$(\roman*)$, align=left, leftmargin=*, labelsep=*, itemindent=*]
	\item $\p \rightarrow (\psi \rightarrow \p \land \psi) $ \hfill (FOL)
	\item $\Wnext (\p \rightarrow (\psi \rightarrow \p \land \psi))$ \hfill ($i$, $\ref{eq:wnextNec}$)
	\item $\Wnext \p \rightarrow \Wnext  (\psi \rightarrow \p \land \psi)$ \hfill ($ii$, $\ref{eq:wnextK}$)
	\item $\Wnext  (\psi \rightarrow \p \land \psi) \rightarrow (\Wnext \psi \rightarrow \Wnext (\p \land \psi))$ \hfill ($\ref{eq:wnextK}$)
	\item $\Wnext \p \rightarrow (\Wnext \psi \rightarrow \Wnext (\p \land \psi))$ \hfill ($iii$, $iv$, FOL)
	\item $\Wnext \p \land \Wnext \psi \rightarrow \Wnext(\p \land \psi)$ \hfill (FOL)
\end{enumerate}

\begin{equation*}
\vdash \Wnext \p \land \Wnext \psi \leftrightarrow \Wnext (\p \land \psi)
\label{eq:wnextandleftright}
\tag{\ref{eq:wnextand}}
\end{equation*}
\begin{enumerate}
[label=$(\roman*)$, align=left, leftmargin=*, labelsep=*, itemindent=*]
	\item $\Wnext (\p \land \psi) \rightarrow \Wnext \p \land \Wnext \psi$ \hfill (\ref{eq:wnextandleft})
	\item $\Wnext \p \land \Wnext \psi \rightarrow \Wnext (\p \land \psi)$ \hfill (\ref{eq:wnextandright})
	\item $\Wnext \p \land \Wnext \psi \leftrightarrow \Wnext (\p \land \psi)$ \hfill ($i$, $ii$, FOL)
\end{enumerate}

\begin{equation}
	\vdash \Next (\p \land \psi) \rightarrow \Next \p \land \Next \psi
\label{eq:nextandright}
\end{equation}
\begin{enumerate}
[label=$(\roman*)$, align=left, leftmargin=*, labelsep=*, itemindent=*]
	\item $\Next (\p \land \psi) \to \Wnext (\p \land \psi)$ \hfill (\ref{eq:nexttownext})
	\item $ \Wnext (\p \land \psi) \to \Wnext \p \land \Wnext \psi$ \hfill (\ref{eq:wnextandleft})
	\item $\Wnext \p \land \Wnext \psi \to ( \Box \bot \lor \Next \p) \land (\Box \bot \lor \Next \psi)$ \hfill (\ref{eq:wnextdef}, FOL)
	\item $\Next (\p \land \psi) \to \lnot \Box \bot$ \hfill (\ref{eq:nexttoboxbot})
	\item $\Next (\p \land \psi) \to ( \Box \bot \lor \Next \p) \land (\Box \bot \lor \Next \psi) \land \lnot \Box \bot$ \hfill ($i$-$iv$, FOL)
	\item $\Next (\p \land \psi) \to \Next \p \land \Next \psi$ \hfill ($v$, FOL)
\end{enumerate}

\begin{equation}
 \vdash \Next \p \land \Next \psi \rightarrow \Next (\p \land \psi) 
\label{eq:nextandleft}
\end{equation}
\begin{enumerate}
[label=$(\roman*)$, align=left, leftmargin=*, labelsep=*, itemindent=*]
	\item $\Next \p \land \Next \psi \to \Wnext \p \land \Wnext \psi$ \hfill (\ref{eq:nexttownext})
	\item $\Wnext \p \land \Wnext \psi \to \Wnext (\p \land \psi)$ \hfill (\ref{eq:wnextandright})
	\item $\Wnext (\p \land \psi) \to \Box \bot \lor \Next (\p \land \psi)$ \hfill (\ref{eq:wnextdef}, FOL)
	\item $\Next \p \land \Next \psi \to \lnot \Box \bot$ \hfill (\ref{eq:nexttoboxbot}, FOL)
	\item $\Next \p \land \Next \psi \to (\Box \bot \lor \Next (\p \land \psi)) \land \lnot \Box \bot$ \hfill ($i$-$iv$, FOL)
	\item $\Next \p \land \Next \psi \to \Next (\p \land \psi)$ \hfill ($v$, FOL)
\end{enumerate}

\begin{equation}
 \vdash \Next \p \land \Next \psi \leftrightarrow \Next (\p \land \psi) 
\tag{\ref{eq:nextand}}
\end{equation}
\begin{enumerate}
[label=$(\roman*)$, align=left, leftmargin=*, labelsep=*, itemindent=*]
	\item $\Next (\p \land \psi) \rightarrow \Next \p \land \Next \psi$ \hfill (\ref{eq:nextandright})
	\item $\Next \p \land \Next \psi \rightarrow \Next (\p \land \psi)$ \hfill (\ref{eq:nextandleft})
	\item $\Next \p \land \Next \psi \leftrightarrow \Next (\p \land \psi) $ \hfill ($i$, $ii$, FOL)
\end{enumerate}

\begin{equation}
	\vdash \Next (\p \lor \psi) \leftrightarrow \Next \p \lor \Next \psi
\label{eq:nextorleftright}
%\tag{\ref{eq:nextor}}
\end{equation}
\begin{enumerate}
[label=$(\roman*)$, align=left, leftmargin=*, labelsep=*, itemindent=*]
	\item $\lnot (\Next \p \lor \Next \psi) \leftrightarrow \lnot \Next \p \land \lnot \Next \psi$ \hfill (FOL)
%	\item $\lnot \Next \p \land \lnot \Next \psi$ \hfill ($i$, FOL)
	\item $\lnot \Next \p \land \lnot \Next \psi  \leftrightarrow \Wnext \lnot \p \land \Wnext \lnot \psi$ \hfill (Def. $\Wnext$)
	\item $\Wnext \lnot \p \land \Wnext \lnot \psi \leftrightarrow \Wnext(\lnot \p \land \lnot \psi)$ \hfill (\ref{eq:wnextandleftright})
	\item $\Wnext (\lnot \p \land \lnot \psi) \leftrightarrow \lnot \Next (\p \lor \psi)$ \hfill (Def. $\Wnext$, FOL)
	\item $\lnot (\Next \p \lor \Next \psi) \leftrightarrow \lnot \Next (\p \lor \psi)$ \hfill ($i$-$iv$, FOL)
	\item $\Next (\p \lor \psi) \leftrightarrow \Next \p \lor \Next \psi$ \hfill ($v$, FOL)
\end{enumerate}

\begin{equation*}
	\vdash \Wnext (\p \lor \psi) \leftrightarrow \Wnext \p \lor \Wnext \psi
\tag{\ref{eq:wnextor}}
\end{equation*}
\begin{enumerate}
[label=$(\roman*)$, align=left, leftmargin=*, labelsep=*, itemindent=*]
	\item $\Wnext (\p \land \psi) \leftrightarrow \Box \bot \lor \Next (\p \lor \psi)$ \hfill $(\ref{eq:wnextdef})$
	\item $\Box \bot \lor \Next (\p \lor \psi) \leftrightarrow \Box \bot \lor (\Next \p \lor \Next \psi)$ \hfill (\ref{eq:nextorleftright}, FOL)
	\item $\Box \bot \lor (\Next \p \lor \Next \psi) \leftrightarrow (\Box \bot \lor \Next \p) \lor (\Box \bot \lor \Next \psi)$ \hfill (FOL)
	\item $(\Box \bot \lor \Next \p) \lor (\Box \bot \lor \Next \psi) \leftrightarrow \Wnext \p \lor \Wnext \psi$ \hfill (FOL)
	\item $\Wnext (\p \land \psi) \leftrightarrow \Wnext \p \lor \Wnext \psi$ \hfill ($i$-$iv$, FOL) 
\end{enumerate}

\begin{equation*}
\vdash \p \Until \psi \rightarrow \Diamond \top
\tag{\ref{eq:untiltotop}}
\end{equation*}
\begin{enumerate}
[label=$(\roman*)$, align=left, leftmargin=*, labelsep=*, itemindent=*]
	\item $\bot \to \lnot \psi$ \hfill (FOL)
	\item $\Box (\bot \to \lnot \psi)$ \hfill ($i$, \ref{eq:boxNec})
	\item $\Box (\bot \to \lnot \psi) \to (\Box \bot \to \Box \lnot \psi)$ \hfill (\ref{eq:boxK})
	\item $\Box \bot \to \Box \lnot \psi$ \hfill ($ii$, $iii$, FOL)
	\item $\Diamond \psi \to \Diamond \top$ \hfill ($iv$, Def.~$\Box$, FOL)
	\item $\p \Until \psi \rightarrow \Diamond \psi$ \hfill (\ref{eq:untiltodiam})
	\item $\p \Until \psi \rightarrow \Diamond \top$ \hfill ($v$, $vi$, FOL)
\end{enumerate}

\begin{equation*}
\text{if $\p \in \monod$, then $\Wnext \p \in \monod$}
\tag{\ref{eq:wnextNec}}
\end{equation*}
\begin{enumerate}
[label=$(\roman*)$, align=left, leftmargin=*, labelsep=*, itemindent=*]
	\item $\p$ \hfill (Ass.)
	\item $\Box \p$ \hfill ($i$, \ref{eq:boxNec})
	\item $\Box \p \to \Wnext \p$ \hfill (\ref{eq:boxdef}, FOL)
	\item $\Wnext \p$ \hfill ($ii$, $iii$, FOL)
\end{enumerate}
